# Supplementary material for: End-to-End Refinement Guided by Pre-trained Prototypical Classifier
Source: arXiv:1805.08698 source file (2018-12-11)

## Supplementary Materials

### The collection of refined X-ray diffraction patterns for different materials

The following figures are shown in vectorgrams. Each of them gives the raw, refined and ground-truth X-ray diffraction patterns. It is recommended to view them in color and zoom in to see the details.

#### Sc1Cu3

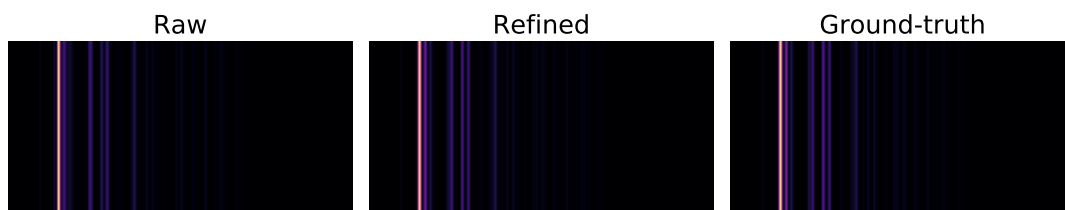

#### Zn3Pt1

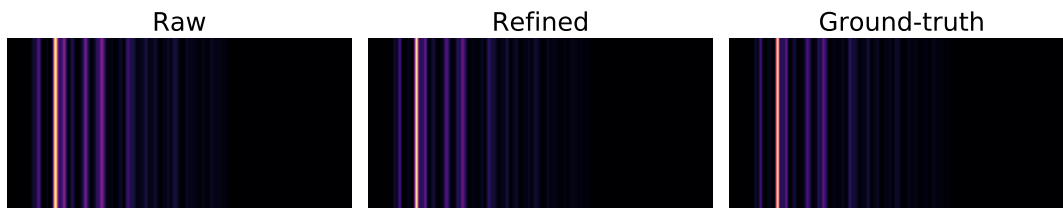

### Yb1Cd3

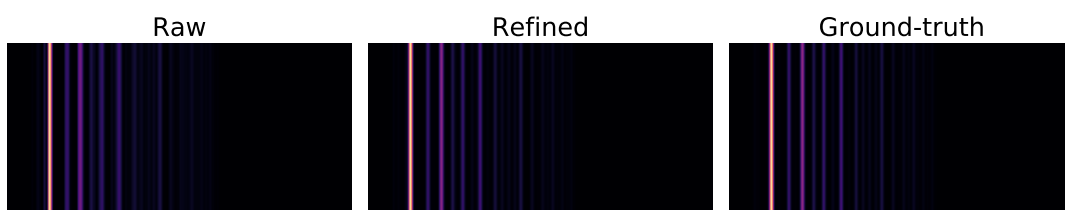

### La1Al2Zn2

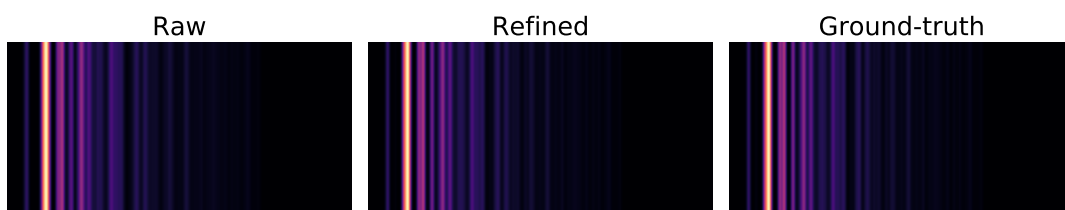

### Li2Al2

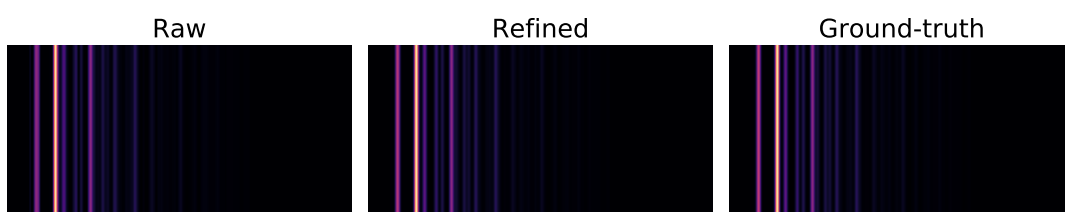

### Cr22Ni50Mo3

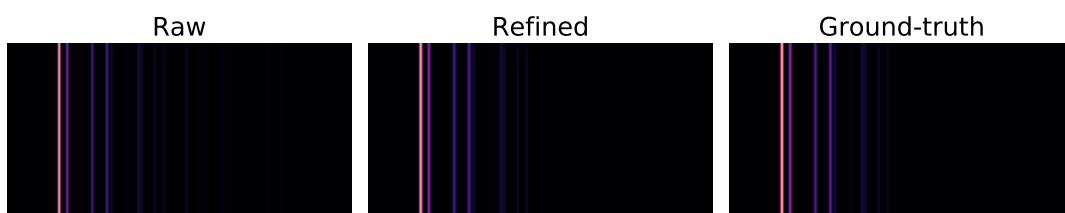

### Bi8Rh4

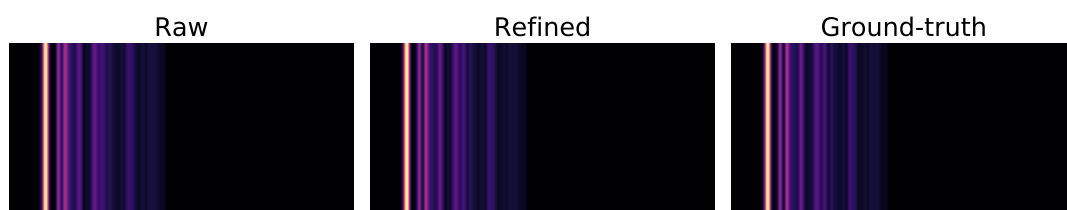

### In12Cu28

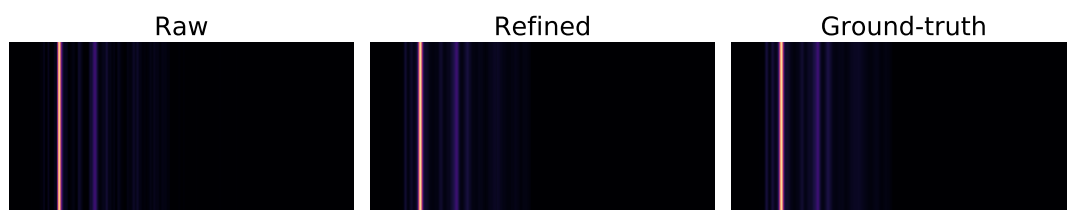

### Lu10Ir4

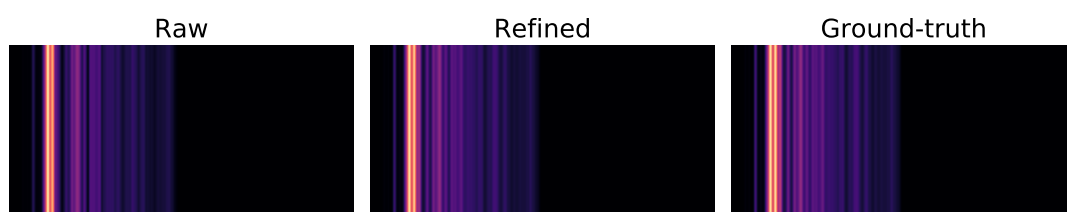

### Nb1Ga3

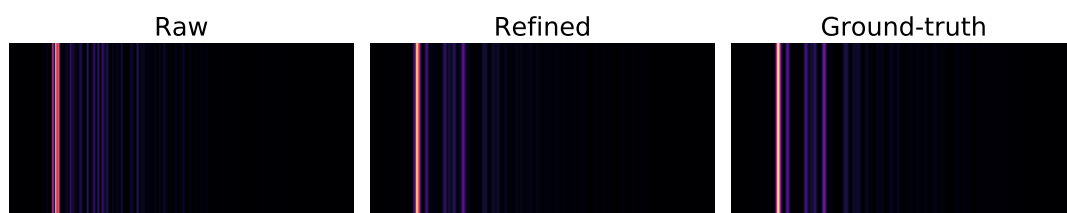

### Y3Co9

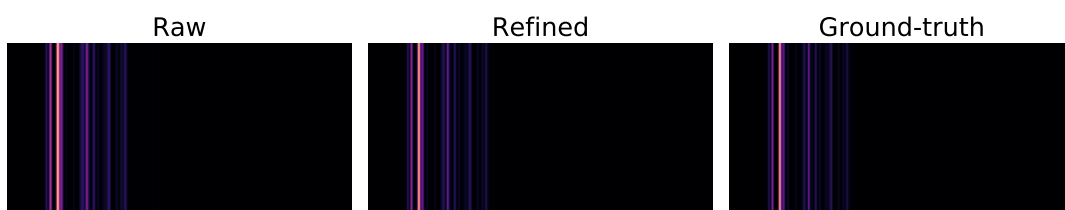

### Pr1Ni5

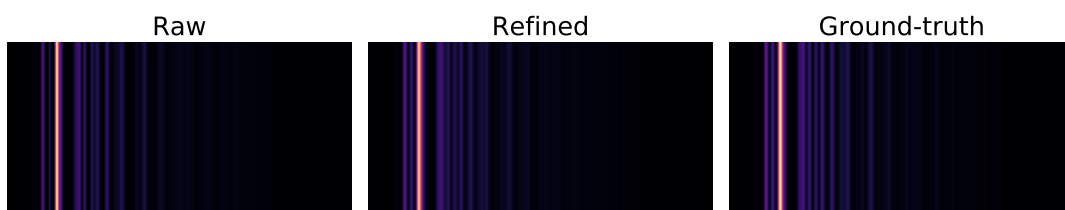

### Mn4Al11

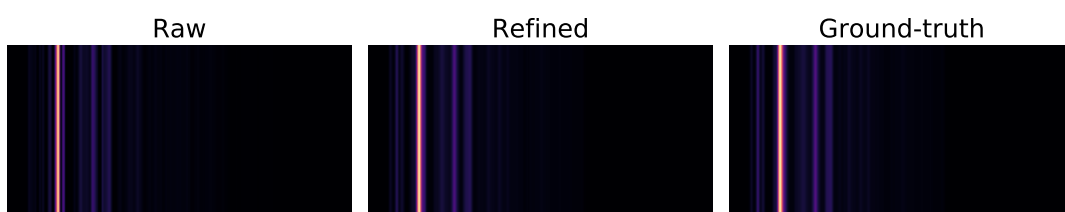

### Bi8Rh4

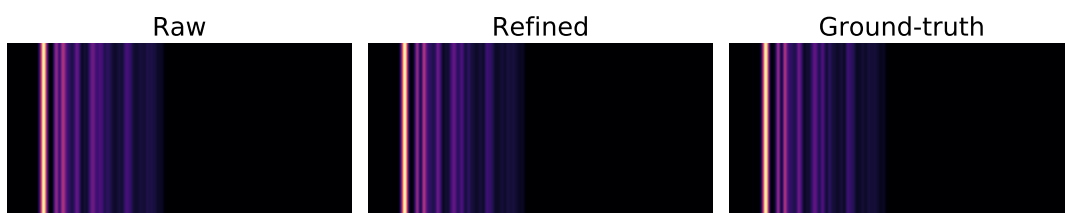

### Ca4Bi2

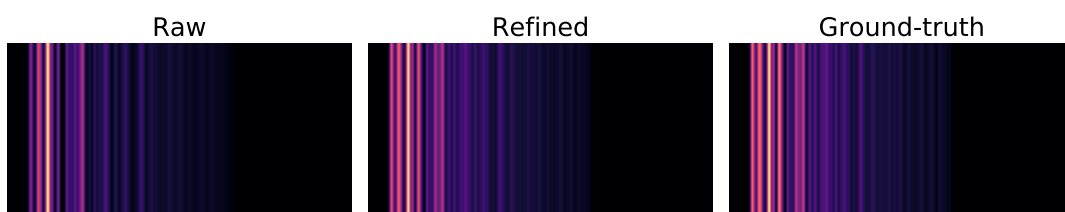

### Zn13Rh1

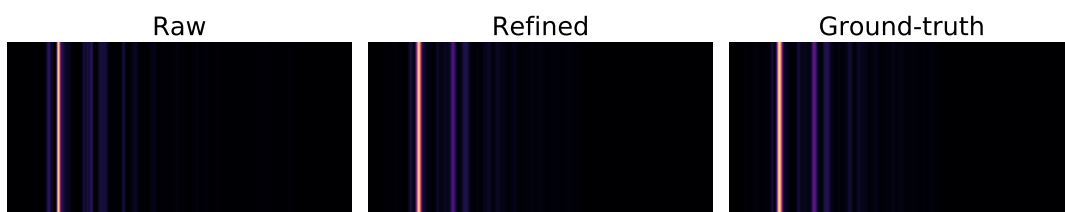

### Ga2Au1

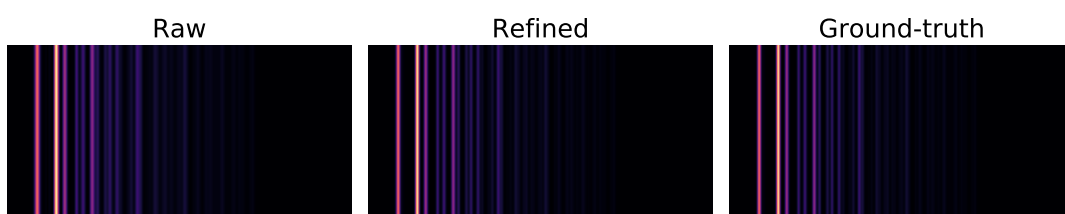

### Li2Ga2

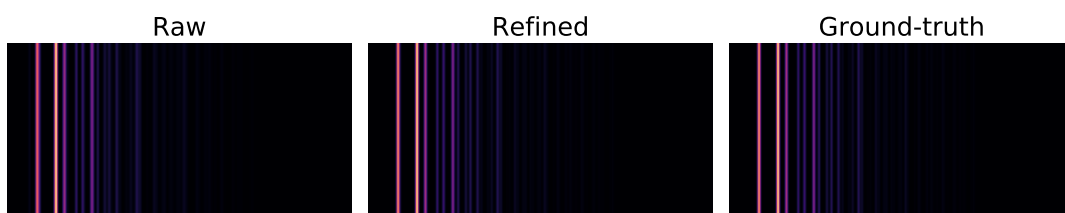

### Sr20Au20

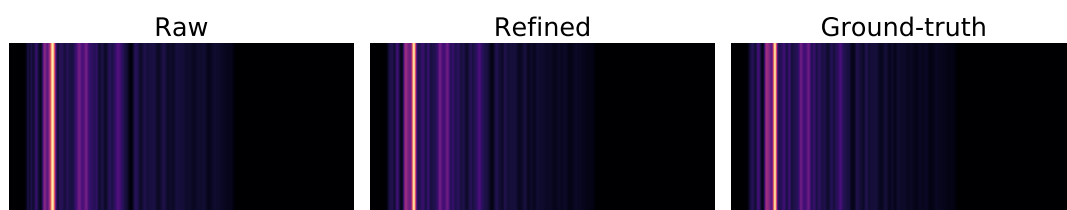

### Nd2Rh2

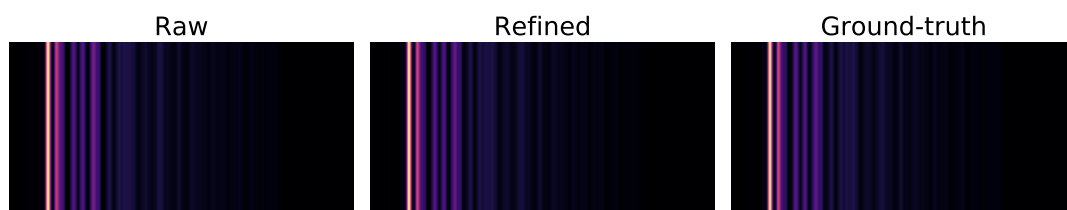

### Dy1Sn1Rh2

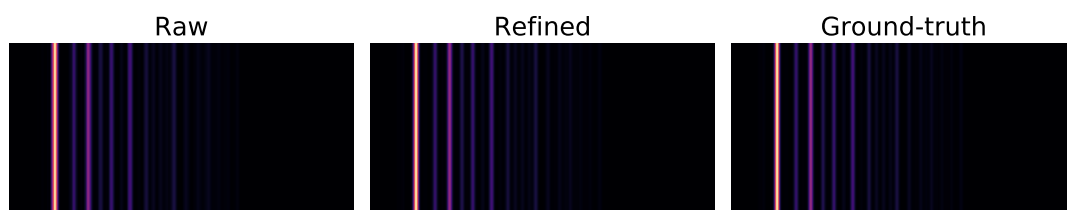

### Li1Al1Ag2

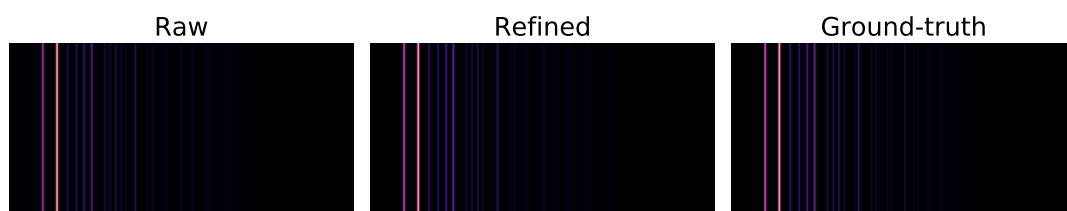

### Bi4Pd10

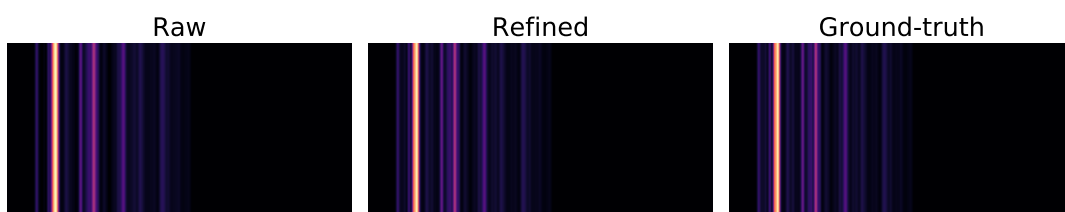

### Co6Mo2

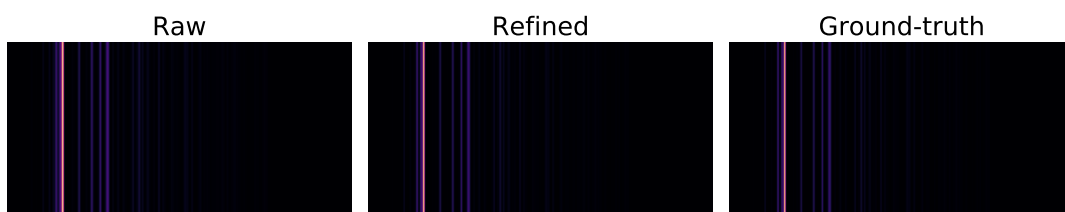

### La4Mg2Ni4

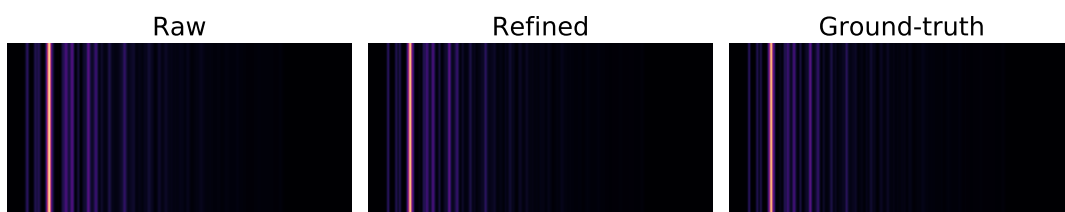

### Sm3Sn3Pt3

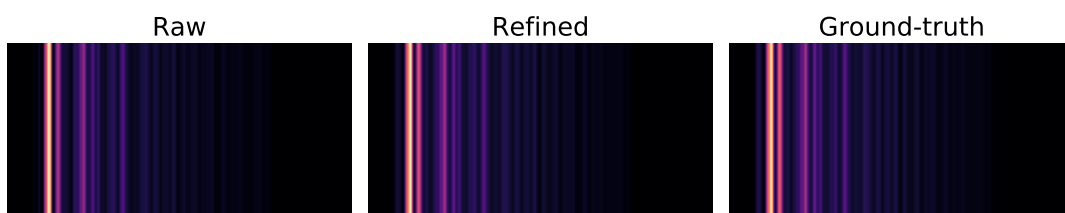

### Sr2In8

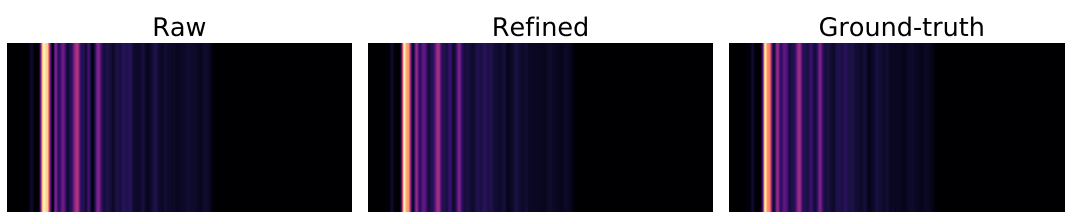

### Y32Co20

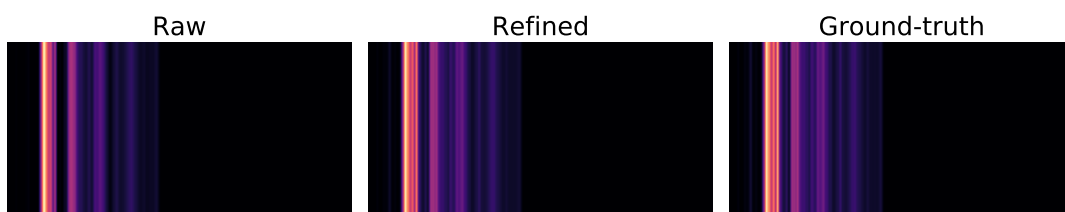

### Ga18Rh4

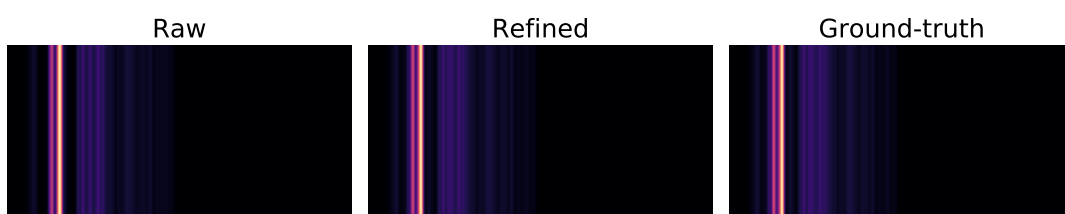

### Pr2Au12

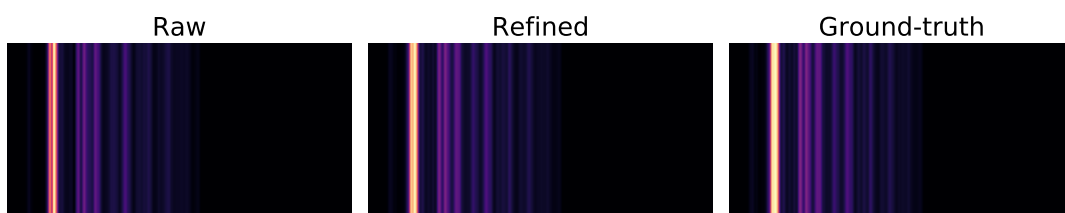



### Mn4Al11

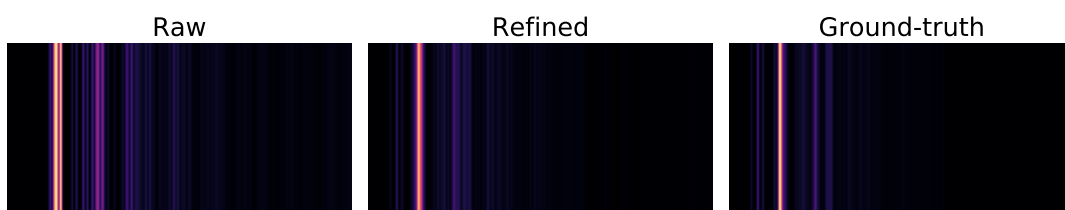

### Cd2

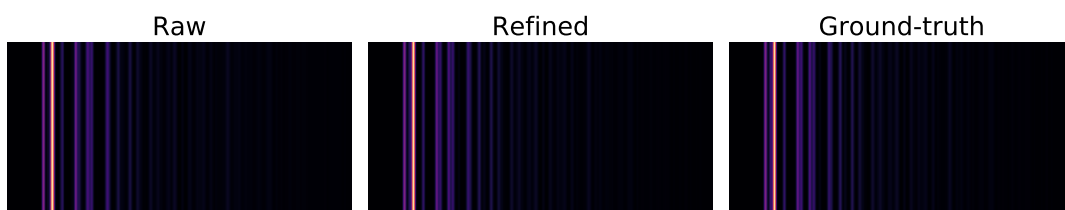

### Pm1Ag3

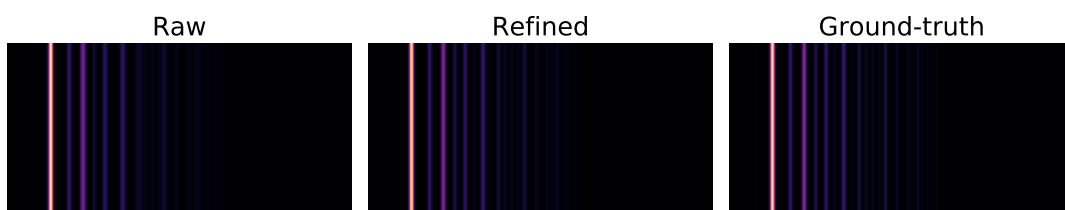

### Mn4Al11

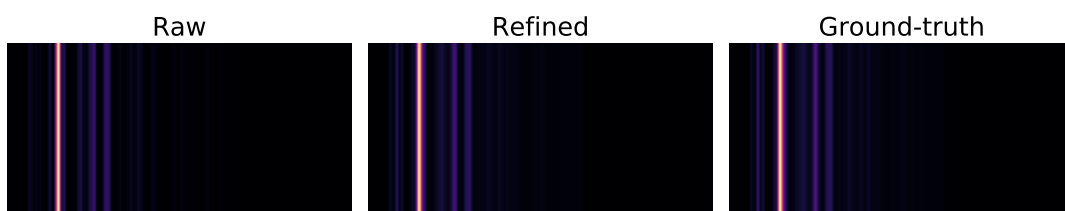

### Eu6Ga4

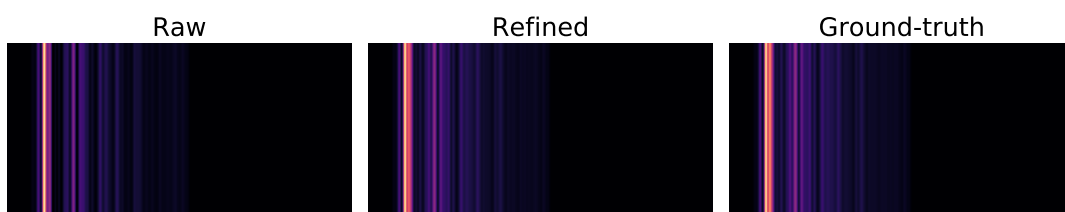

### Pr2Au12

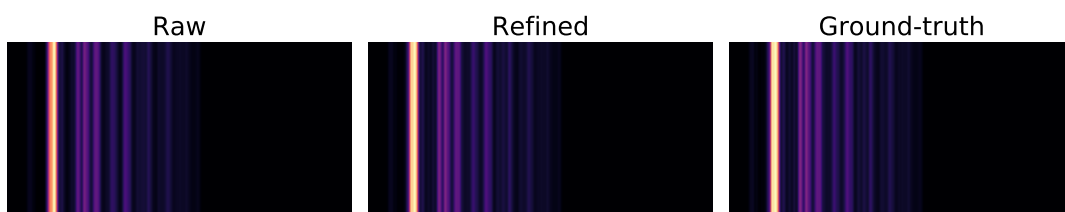

### Nd4Al4Pt4

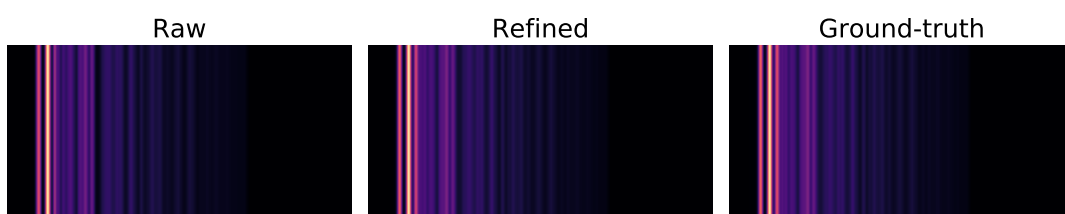

### Zr2Ni6

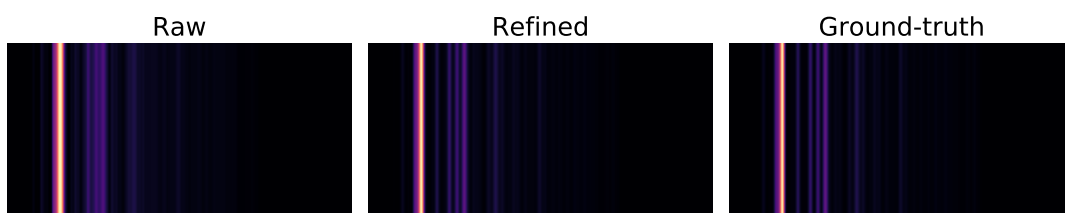

## Pr1Co5

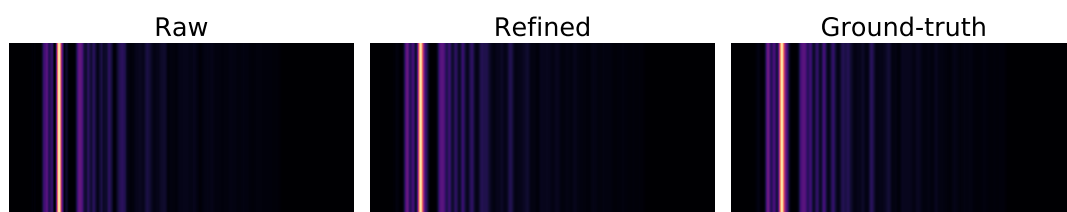

## Lu10Ir4

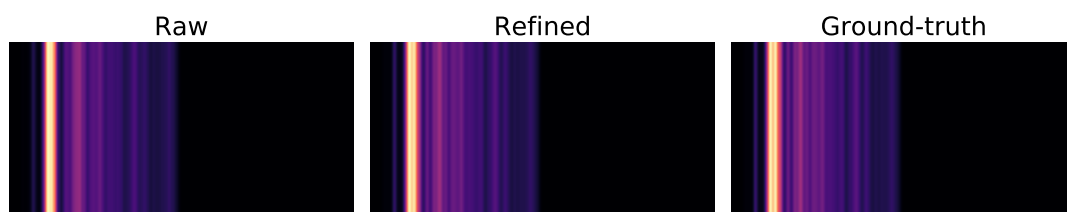

Supplement: Supplementary file 1 [file supp.pdf]
